# Supplementary material for: Metadata-Driven Federated Learning of Connectional Brain Templates in Non-IID Multi-Domain Scenarios
Source: arXiv:2403.09139 source file (2024-03-14)

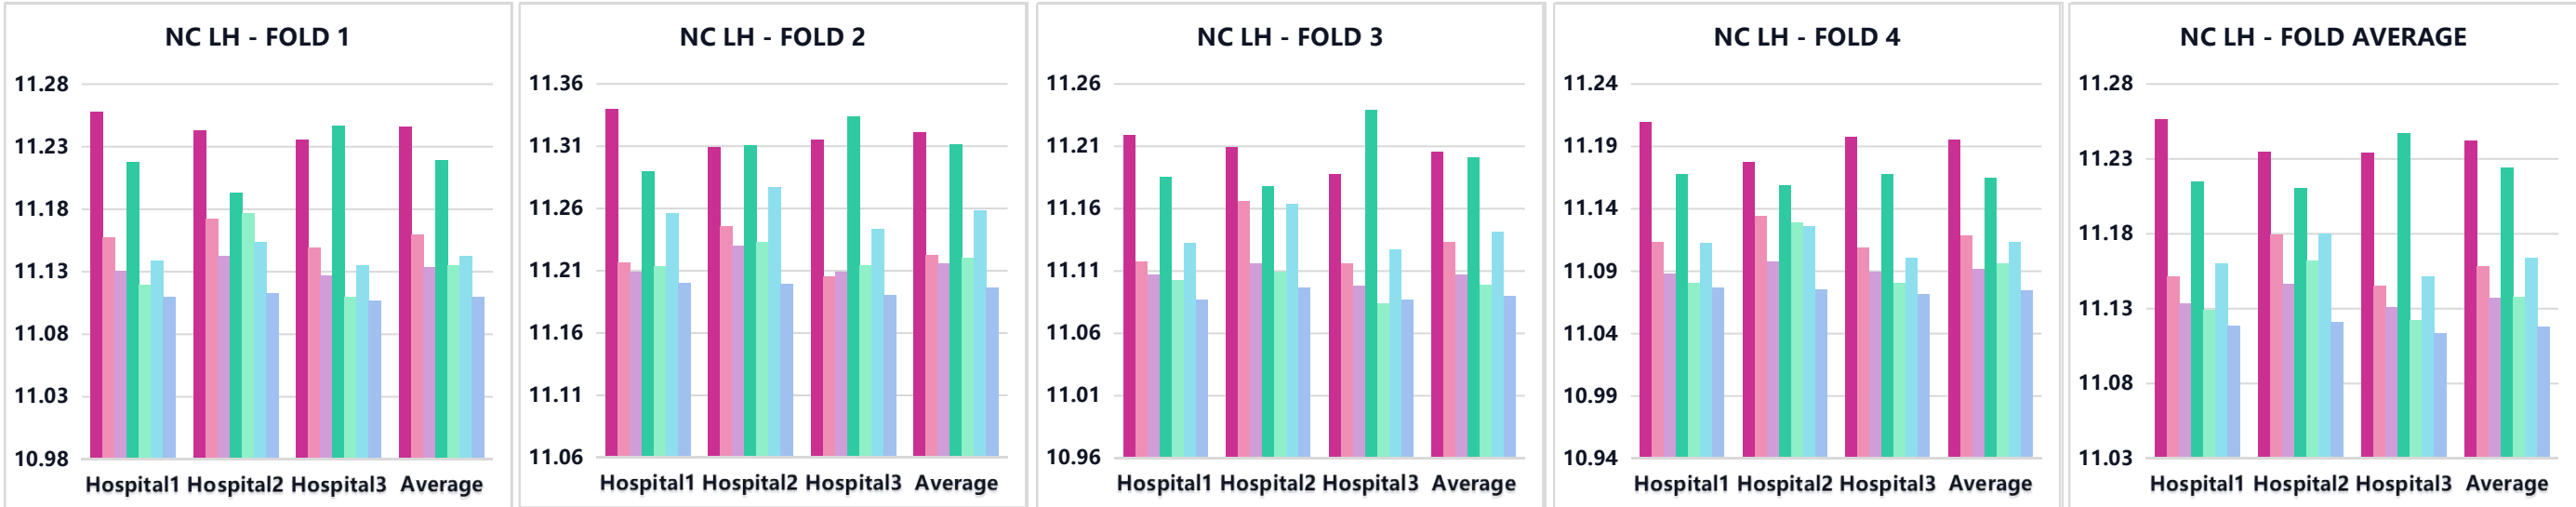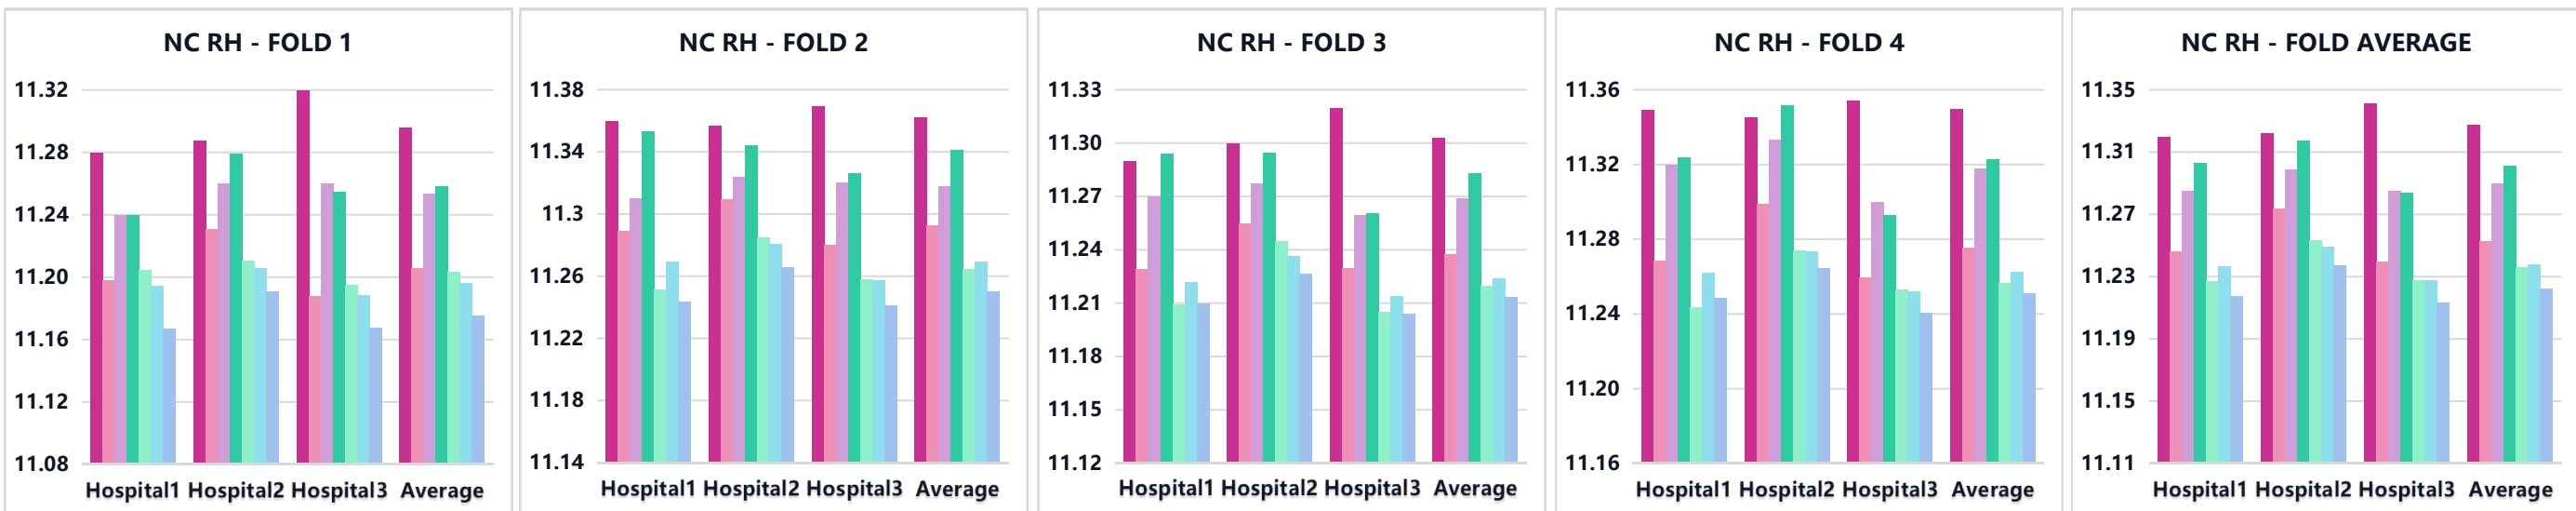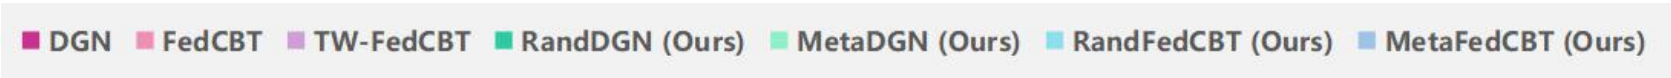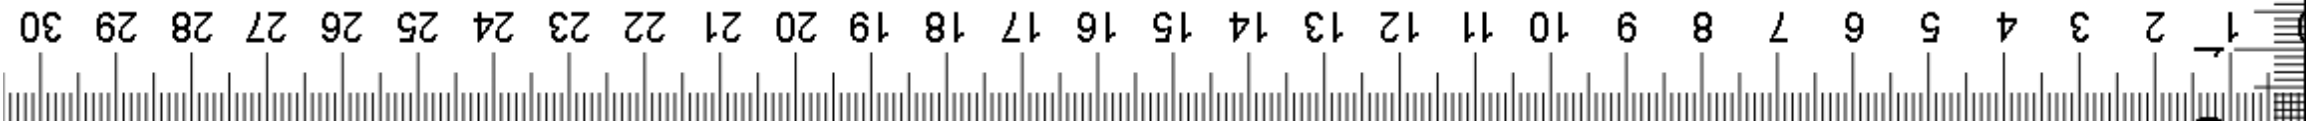

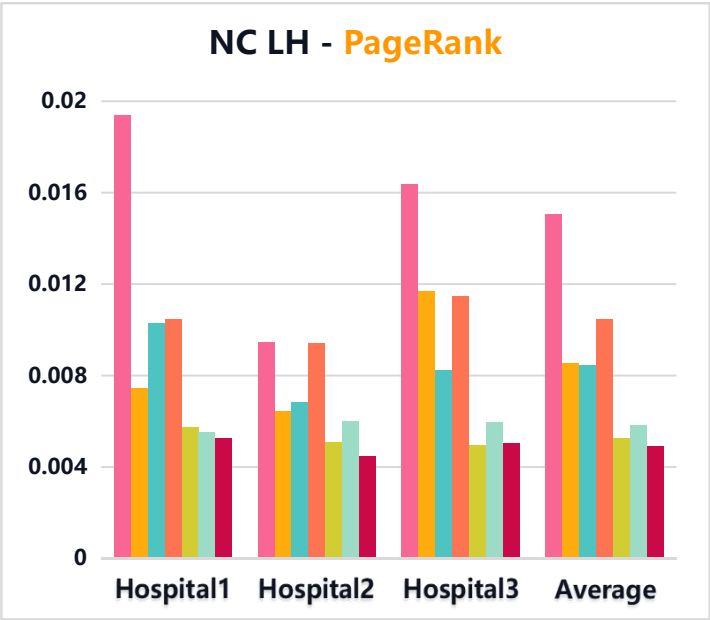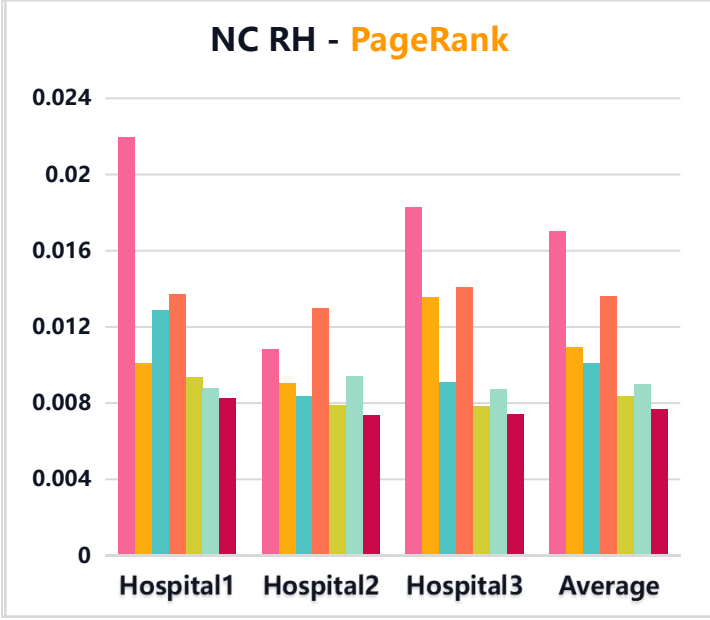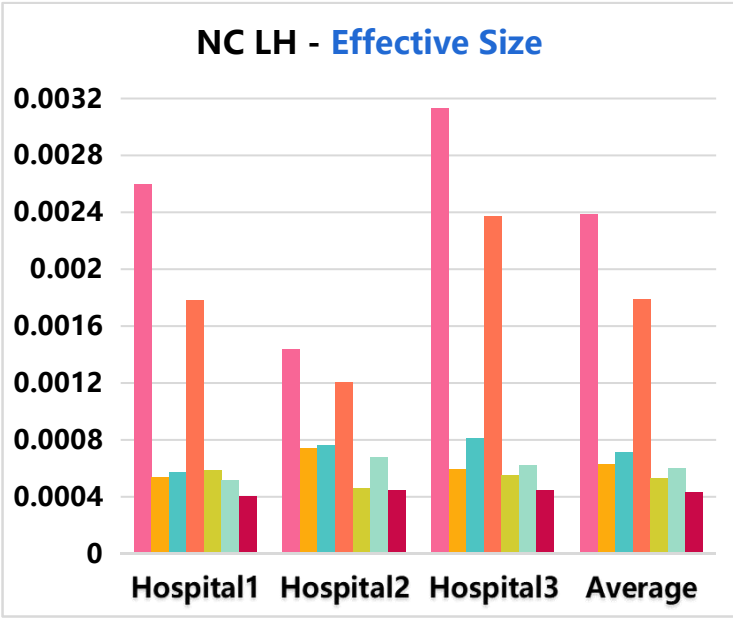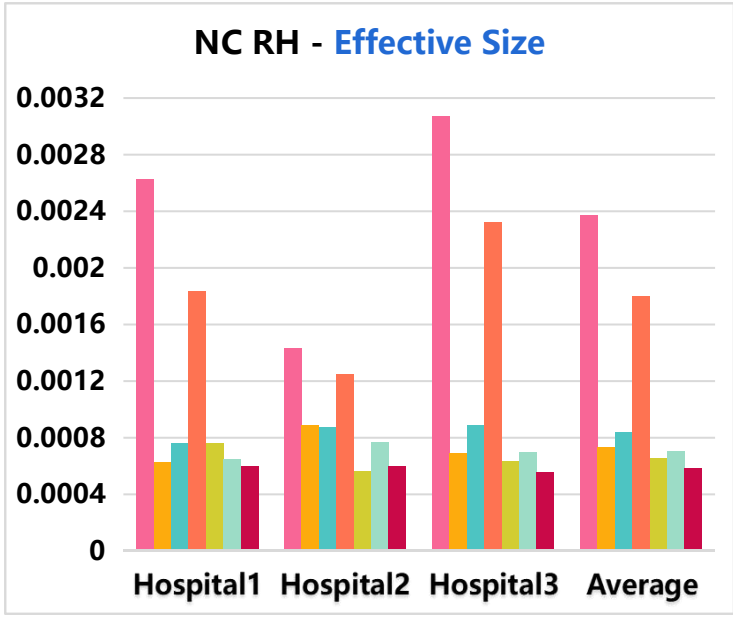

DGN FedCBT TW-FedCB RandDGN (Ours) MetaDGN (Ours) RandFedCBT (Ours) MetaFedCBT (Ours)

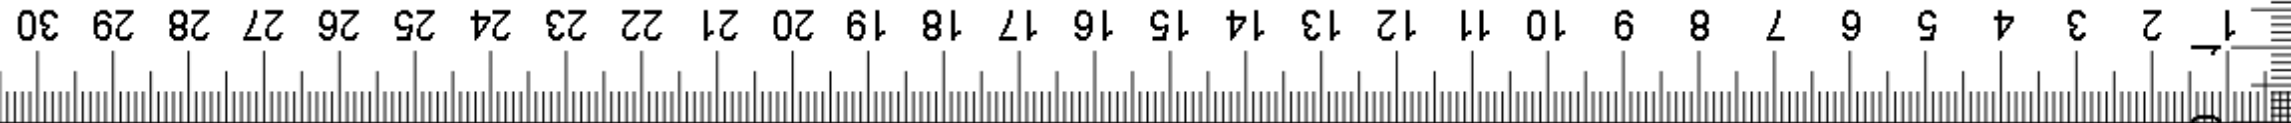

Supplement: Supplementary file 1 [file Results_supp.pdf]
