# Supplementary material for: Metadata-Driven Federated Learning of Connectional Brain Templates in Non-IID Multi-Domain Scenarios
Source: arXiv:2403.09139 source file (2024-03-14)

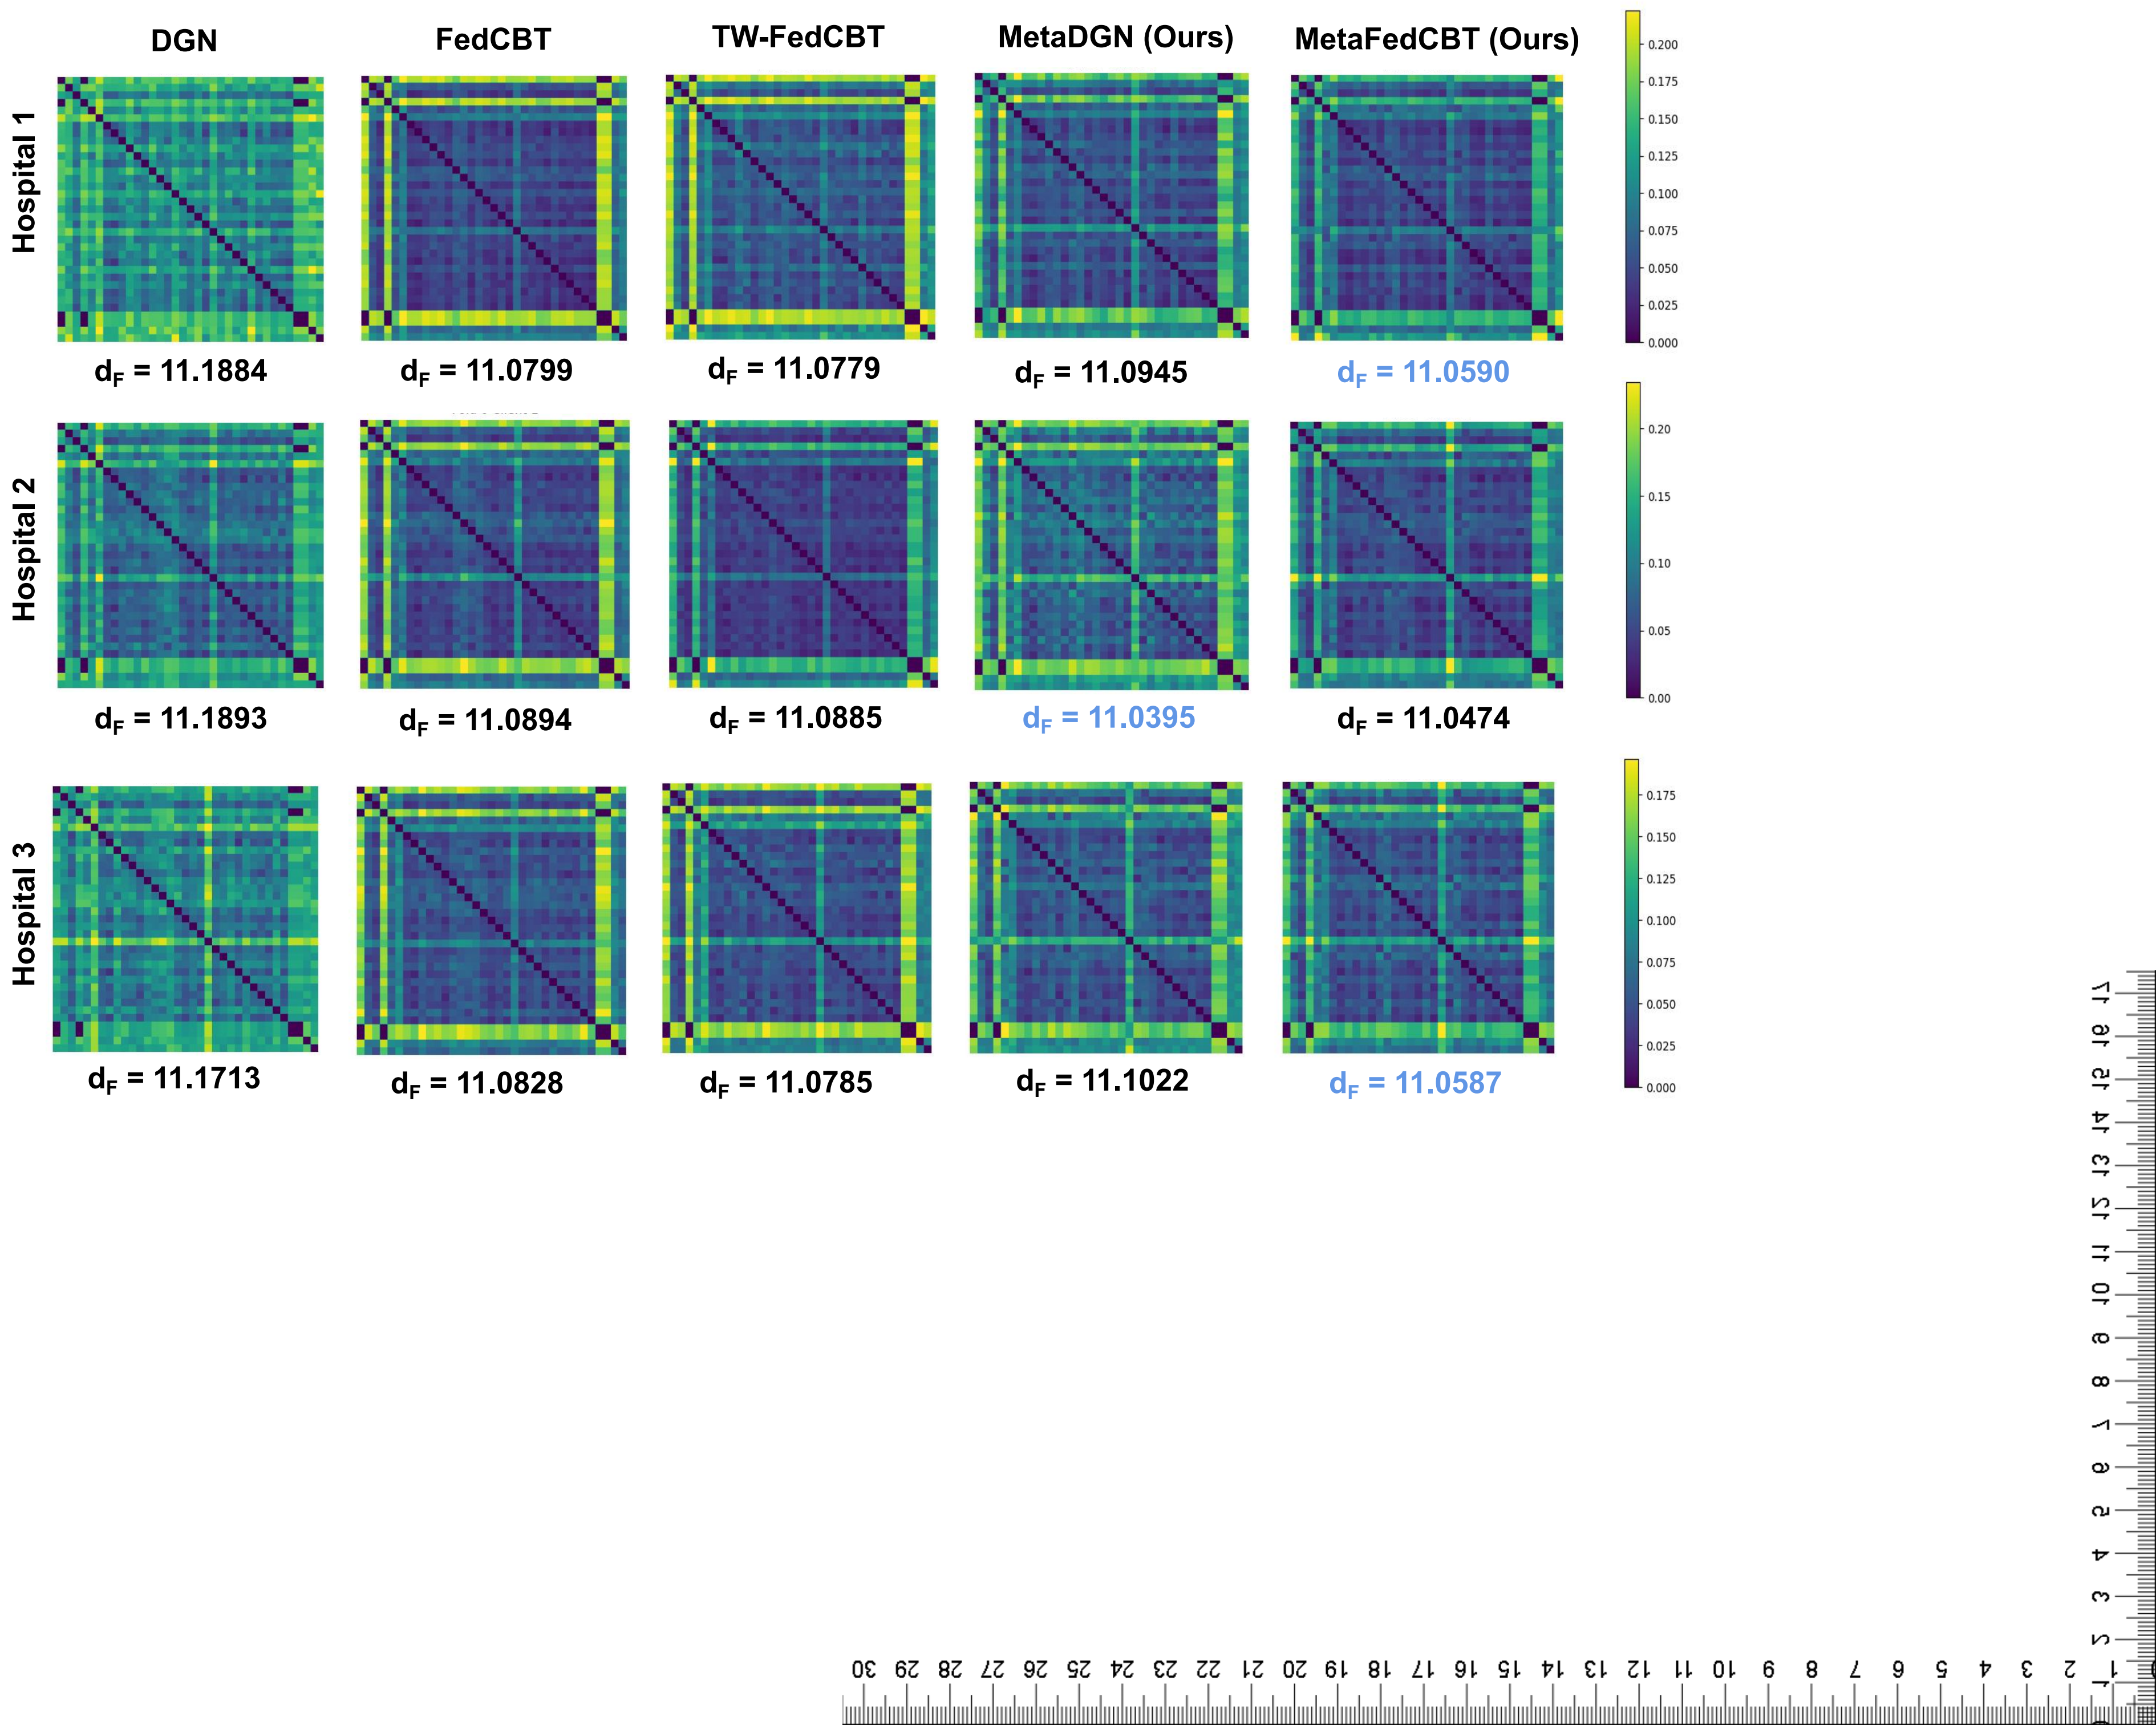



Hospital 1

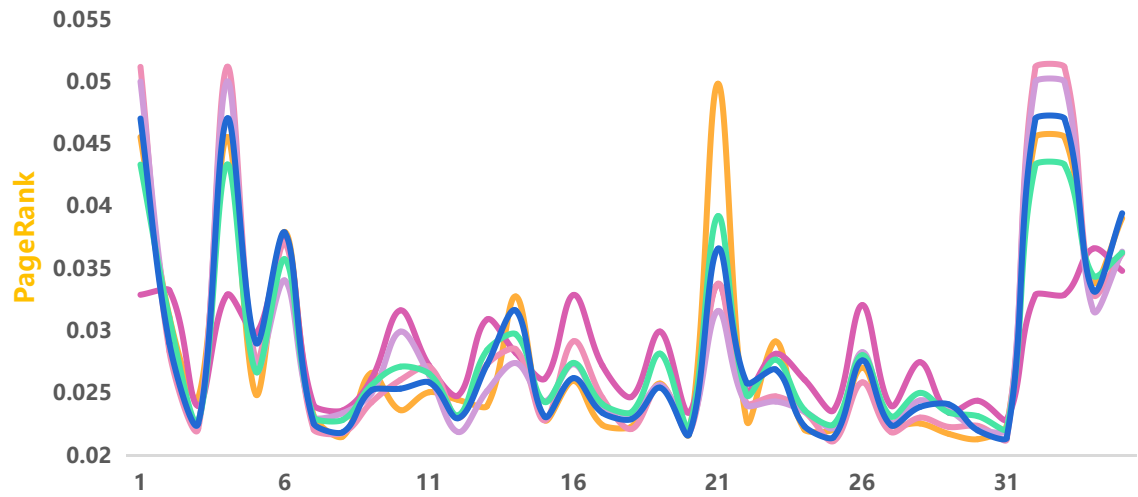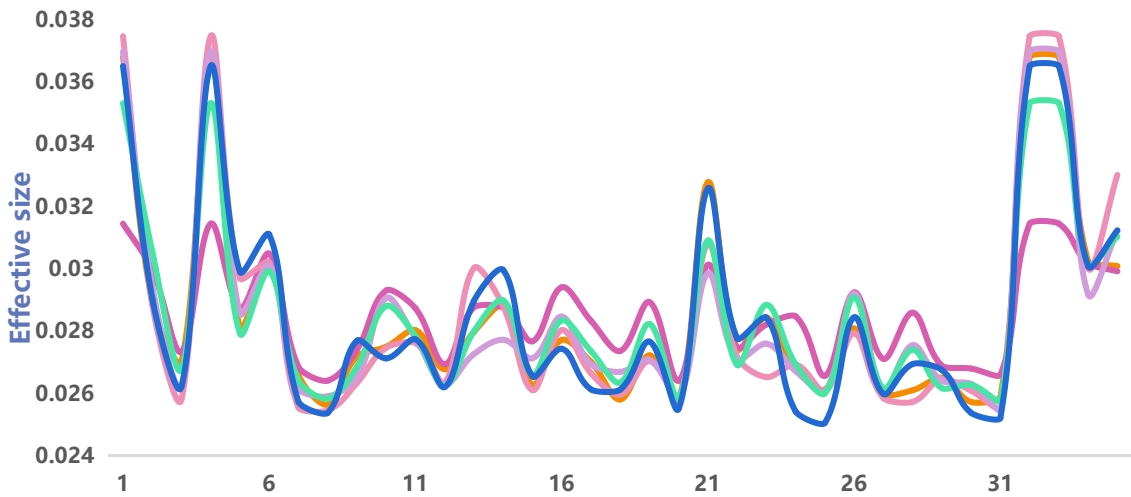

Hospital 2

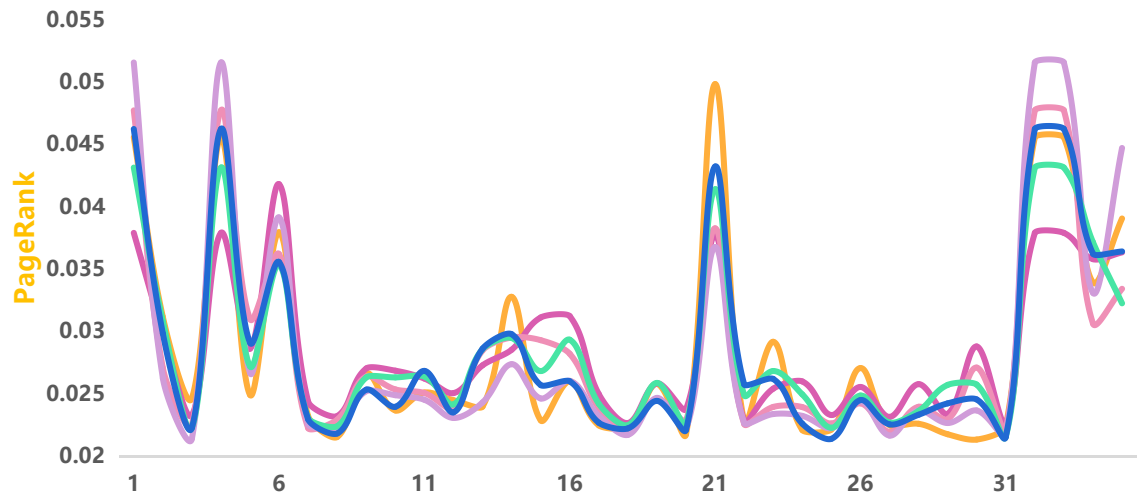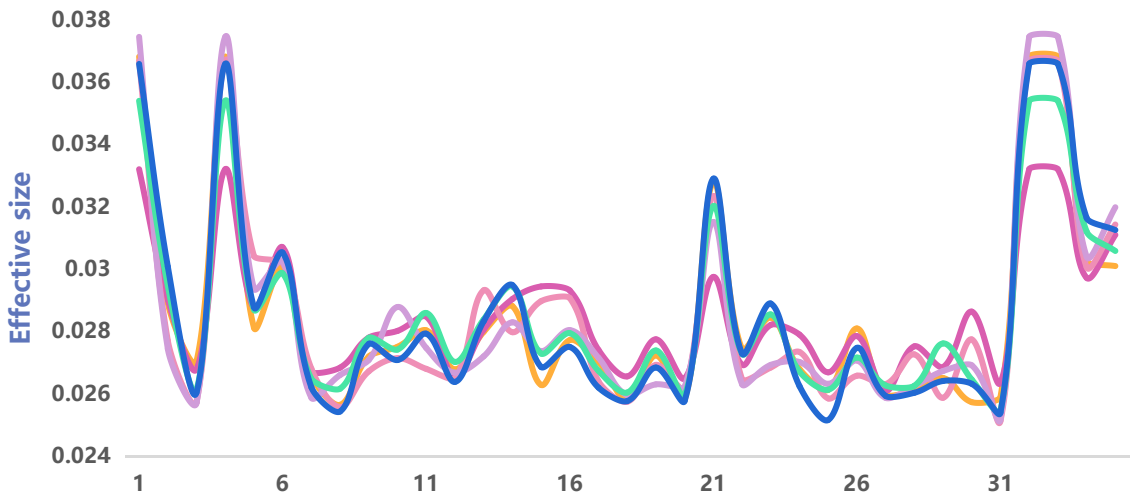

Hospital 3

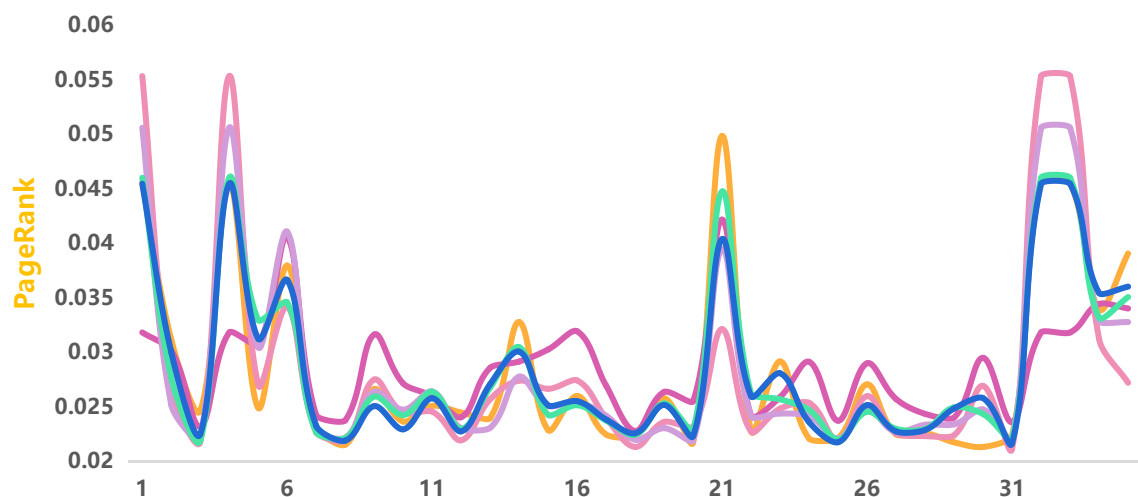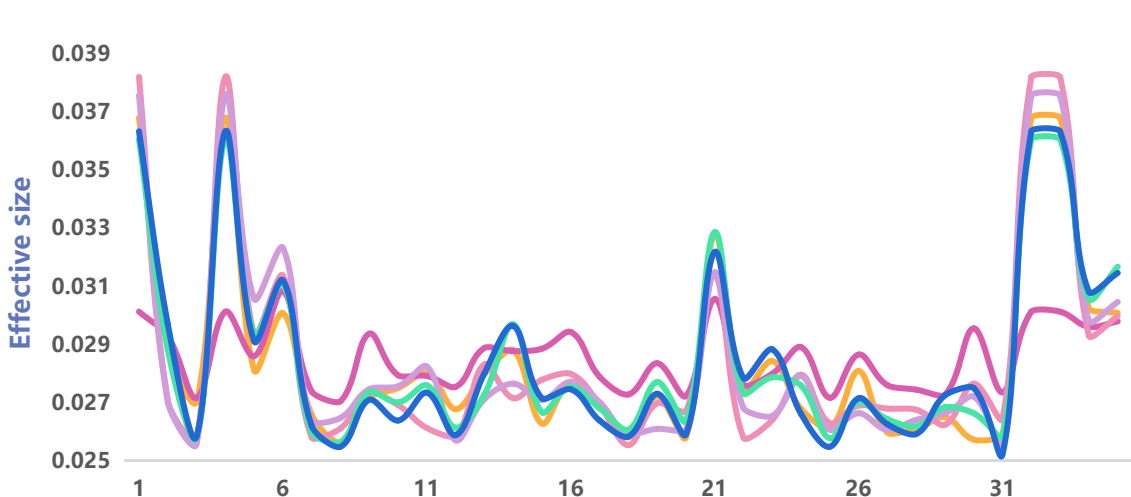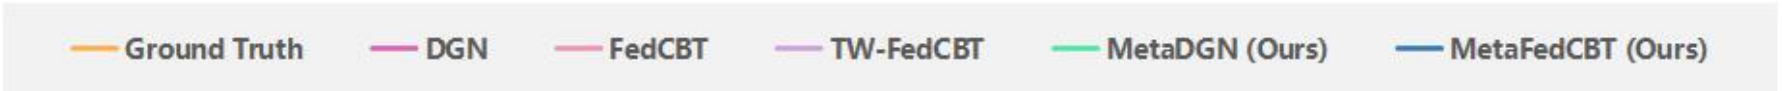

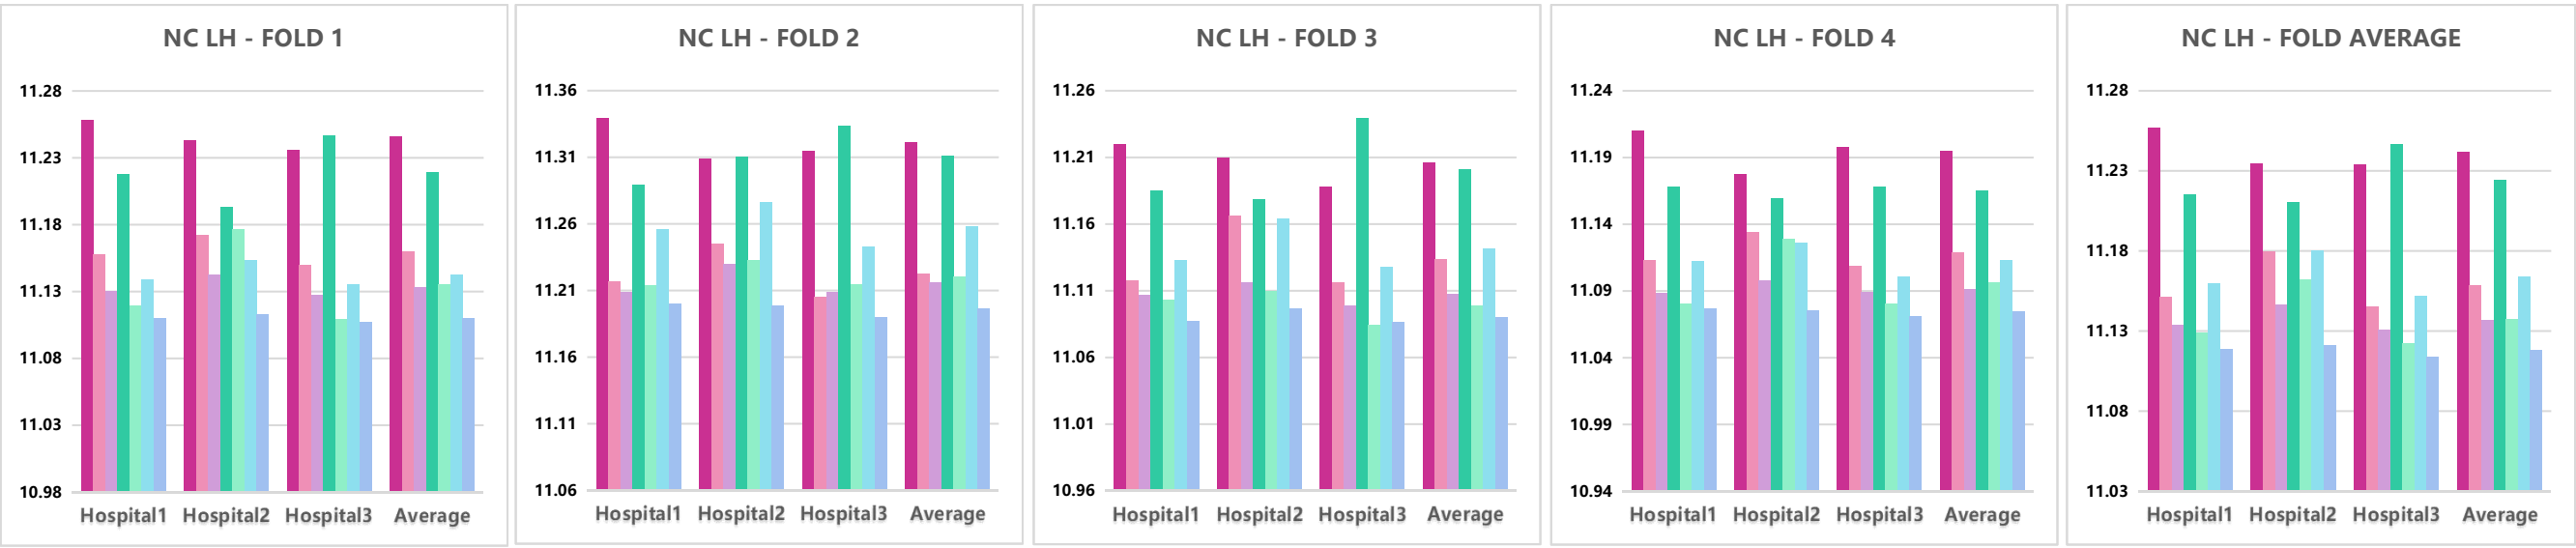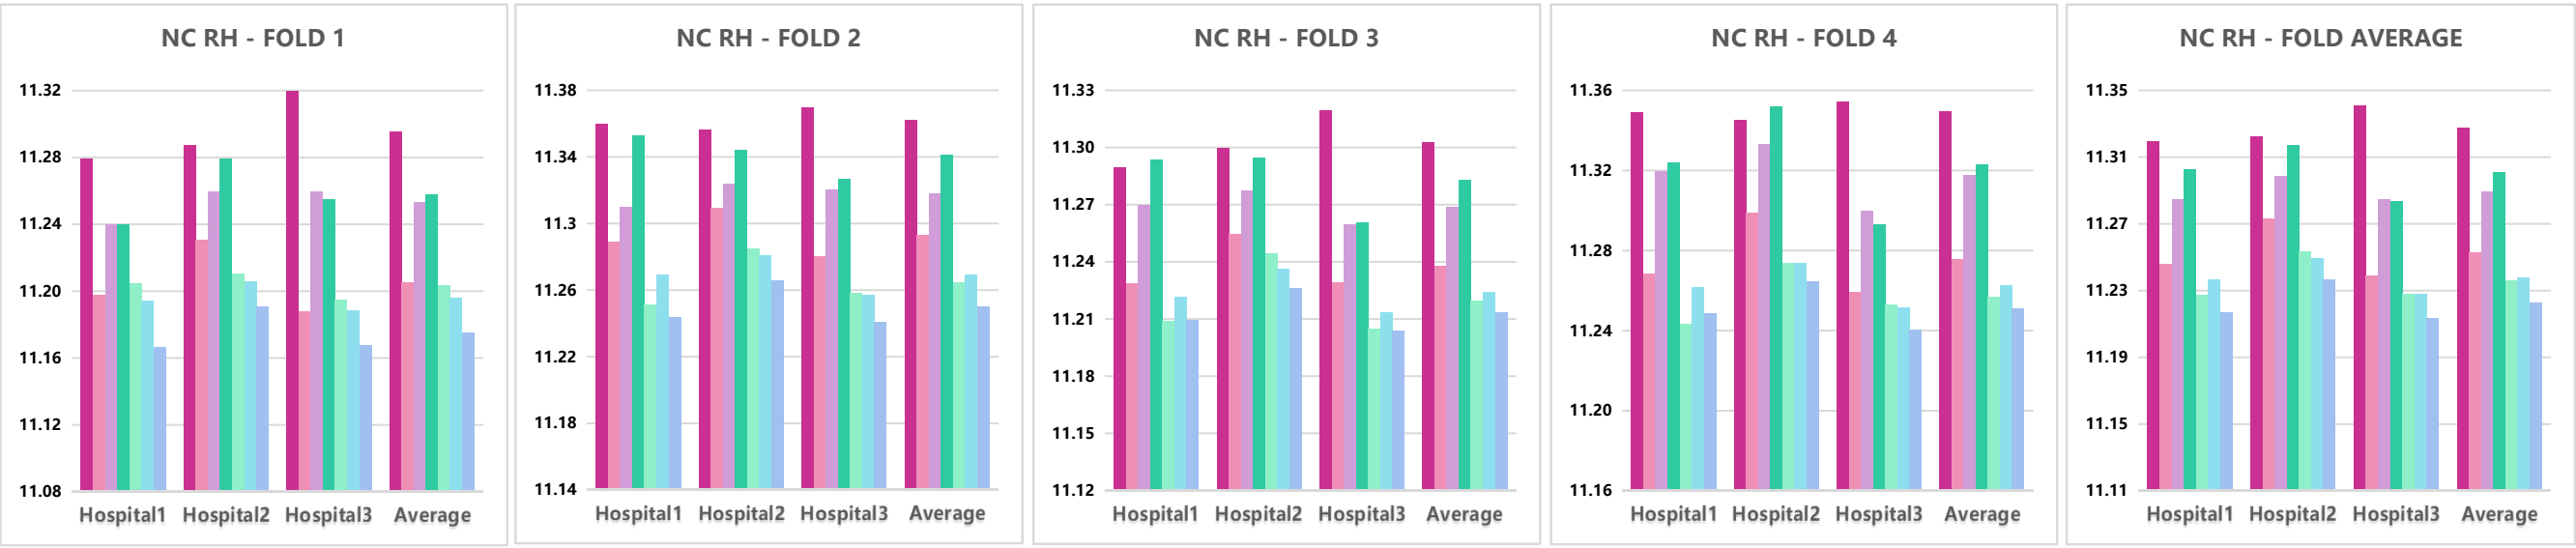

DGN FedCBT TW-FedCBT RandDGN (Ours) MetaDGN (Ours) RandFedCBT (Ours) MetaFedCBT (Ours)

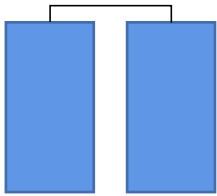

\*\*\*\*  
\*\*\*\*  
\*\*\*\*  
\*\*\*  
\*\*\*  
\*\*\*  
\*\*\*

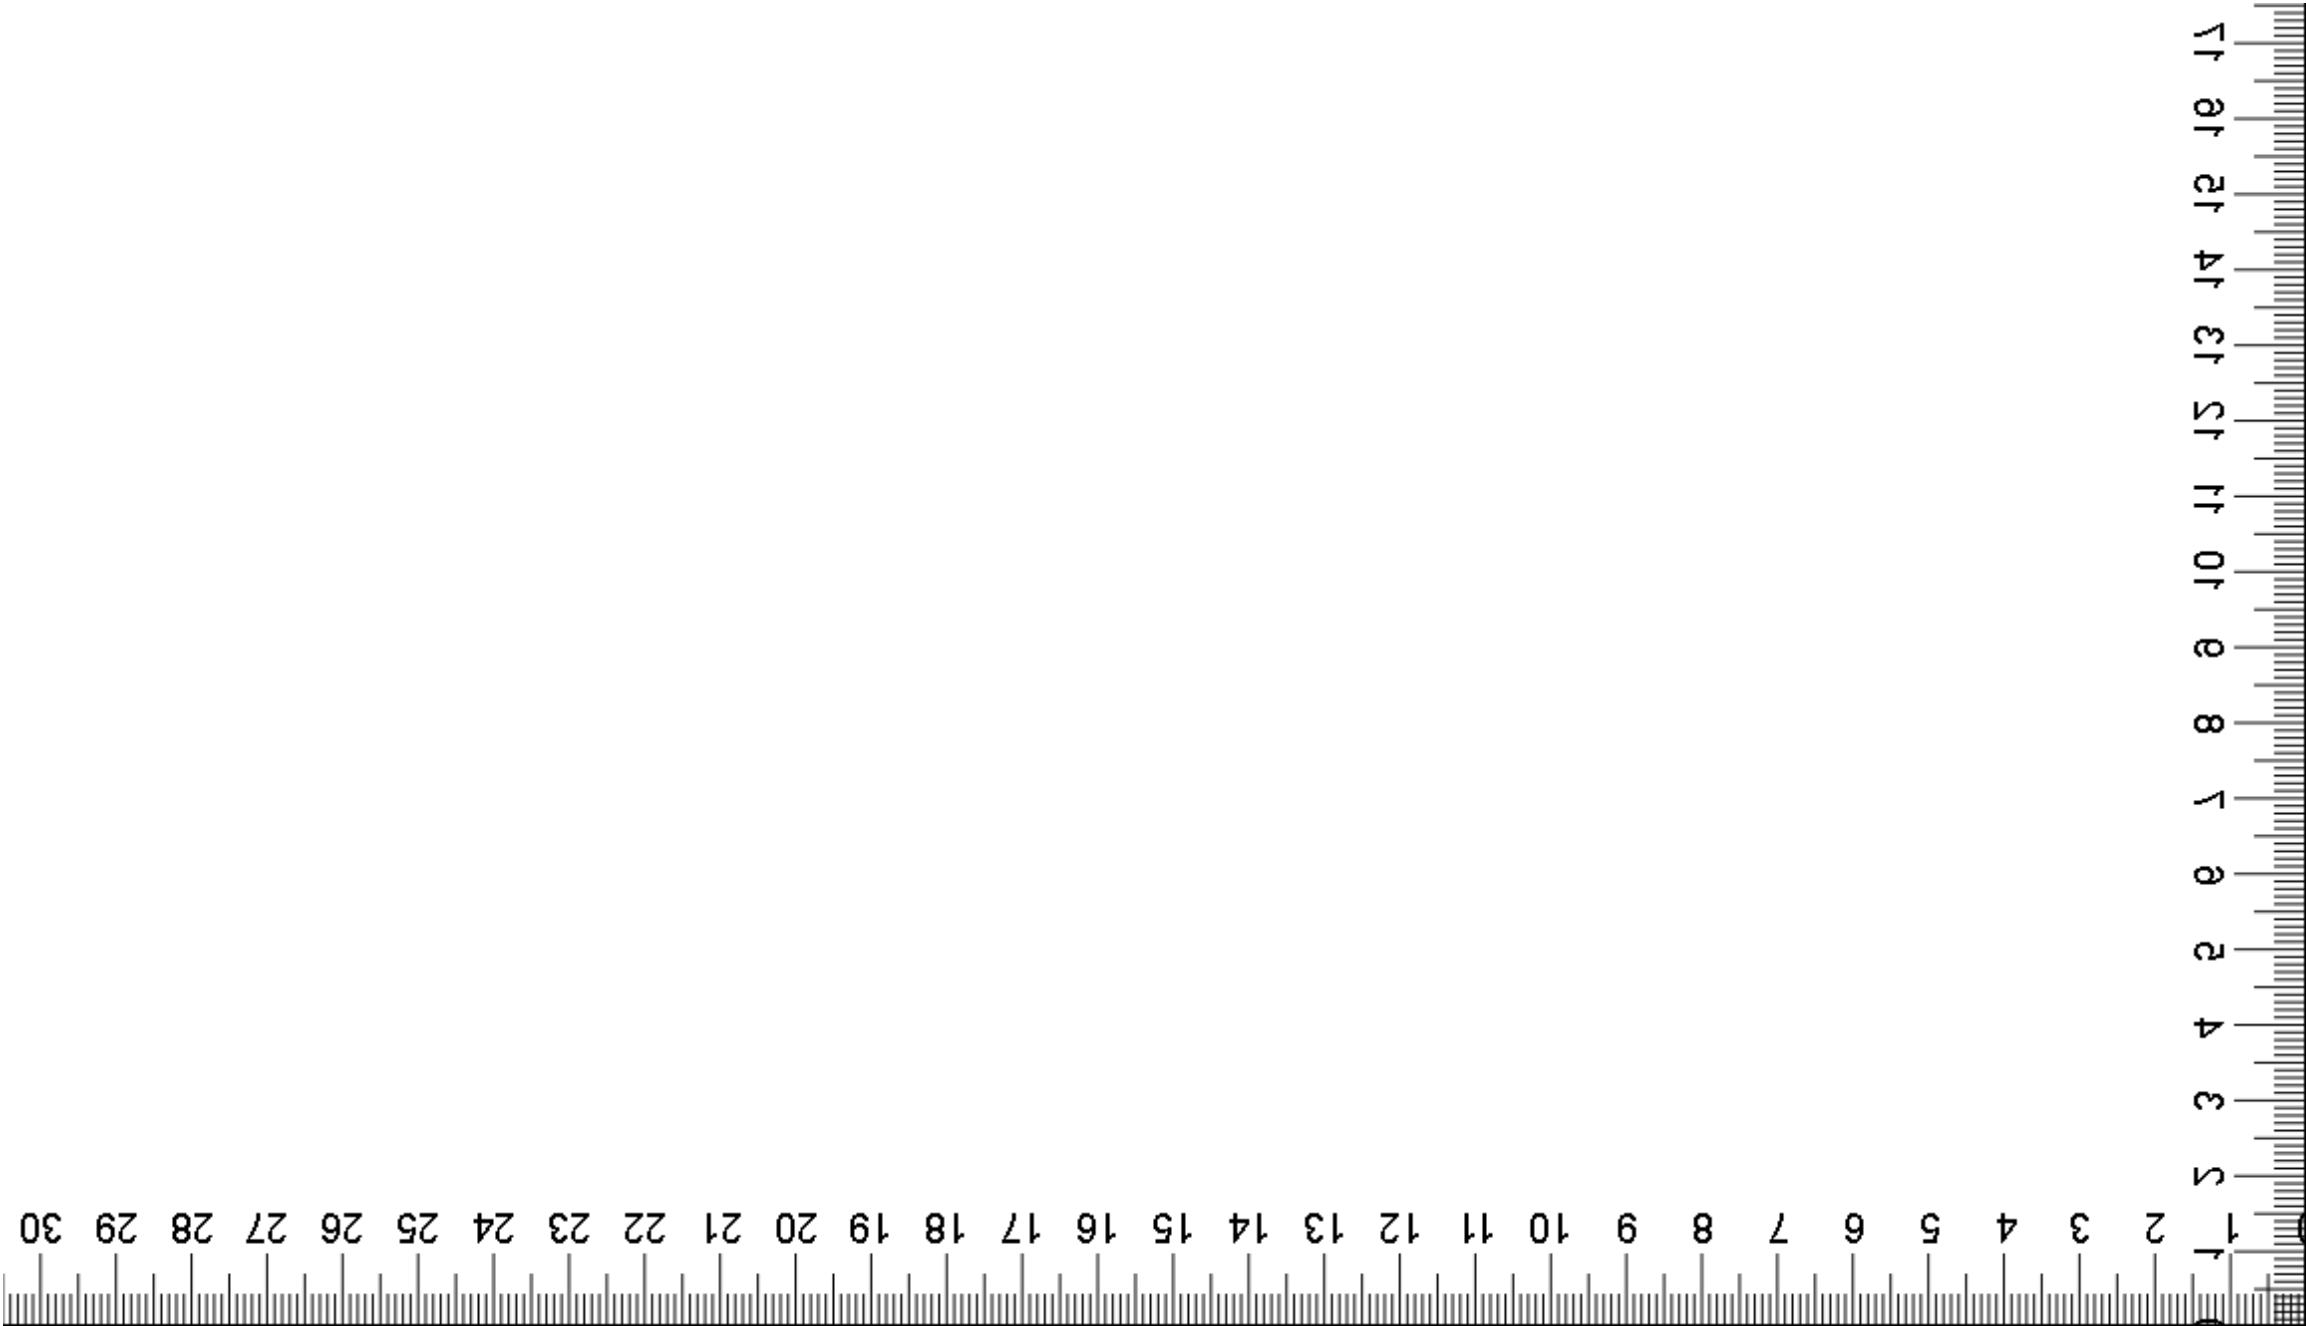

PageRank

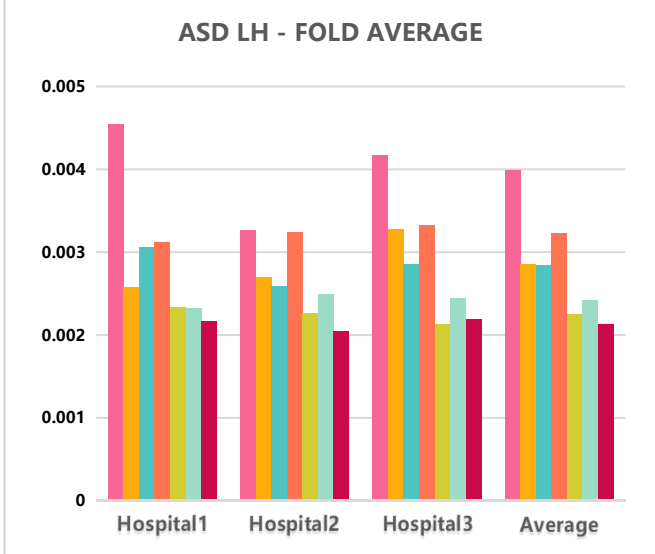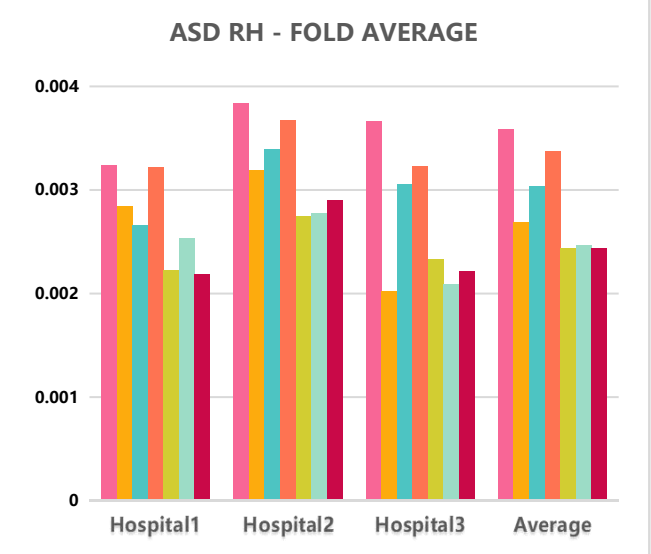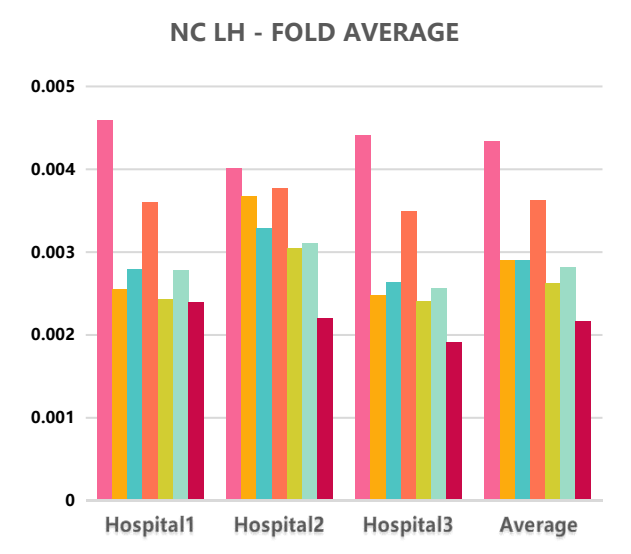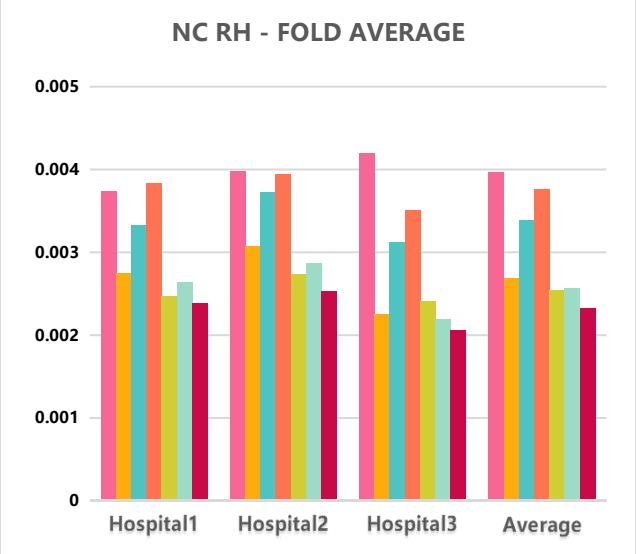

Effective size

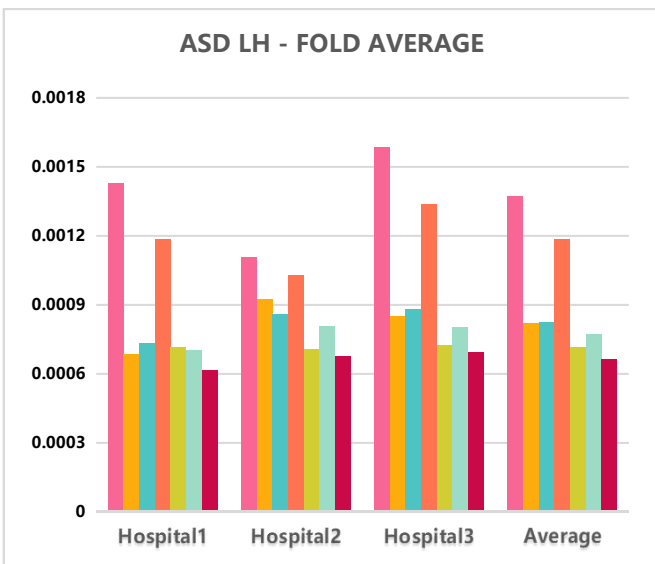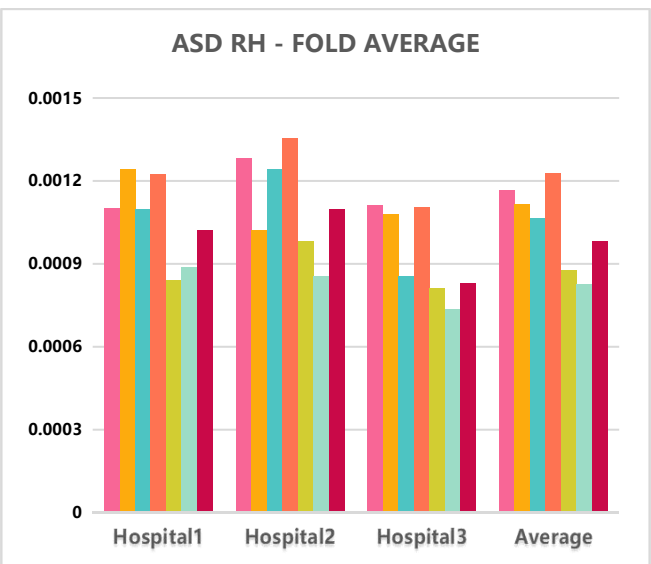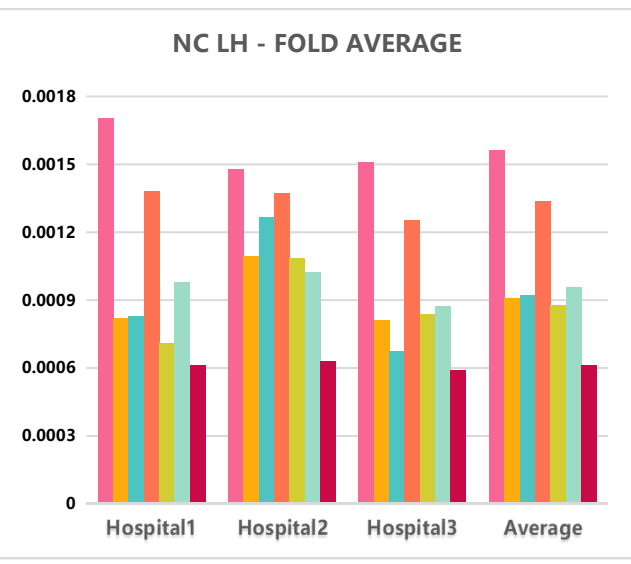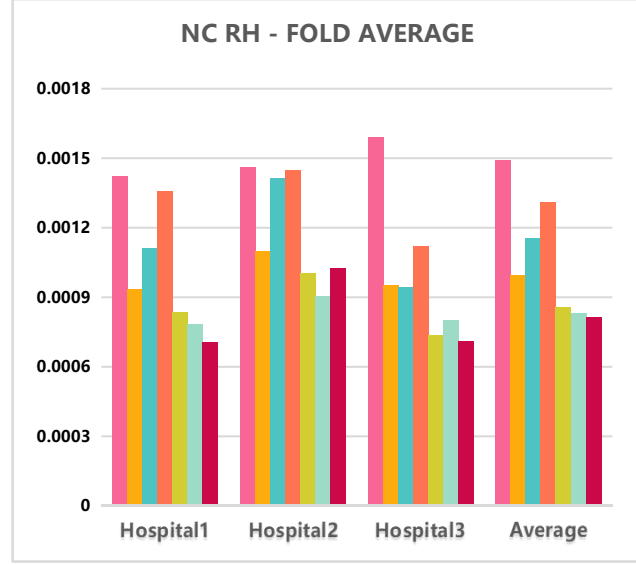

DGN-CBT FedDGN-CBT TW-FedDGN-CBT RandDGN-CBT(Ours) MetaDGN-CBT(Ours) RandFed-CBT(Ours) MetaFed-CBT(Ours)

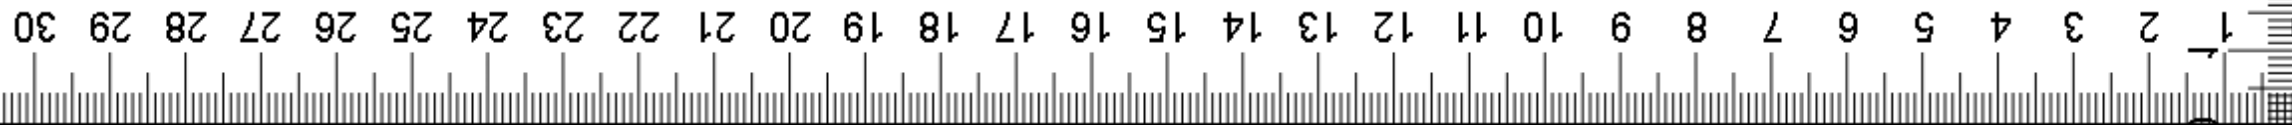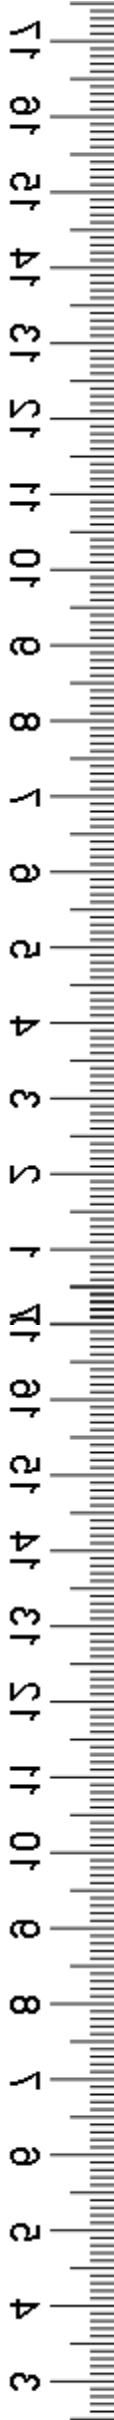

Supplement: Supplementary file 2 [file Results_supp_hospital.pdf]
