# Supplementary material for: Metadata-Driven Federated Learning of Connectional Brain Templates in Non-IID Multi-Domain Scenarios
Source: arXiv:2403.09139 source file (2024-03-14)

**ASD RH FOLD 1**

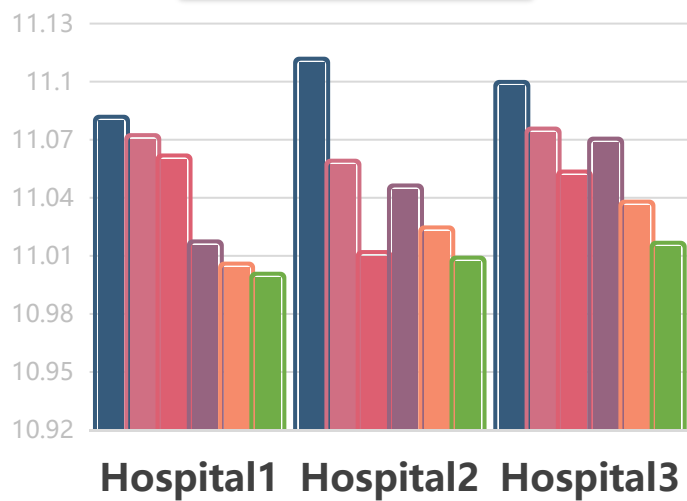

**ASD RH FOLD 2**

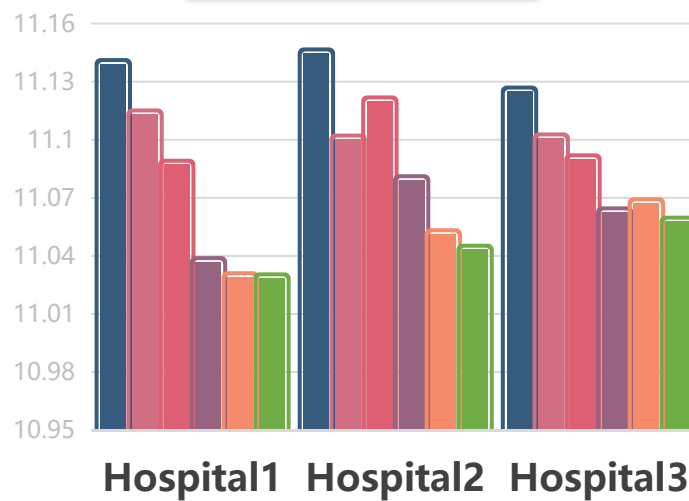

**ASD RH FOLD 3**

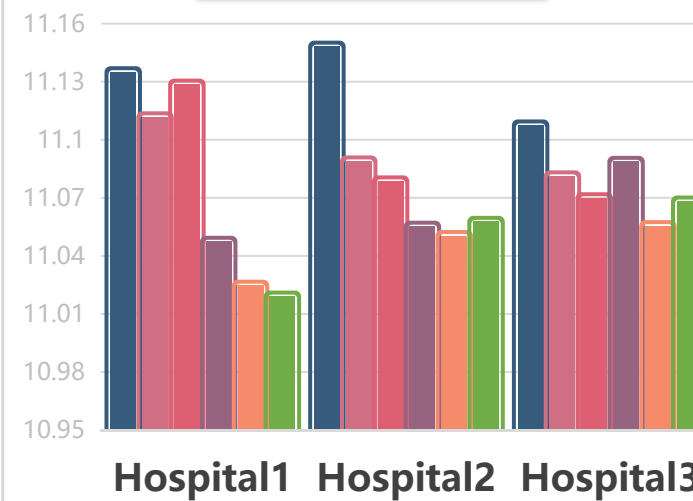

**ASD RH FOLD 4**

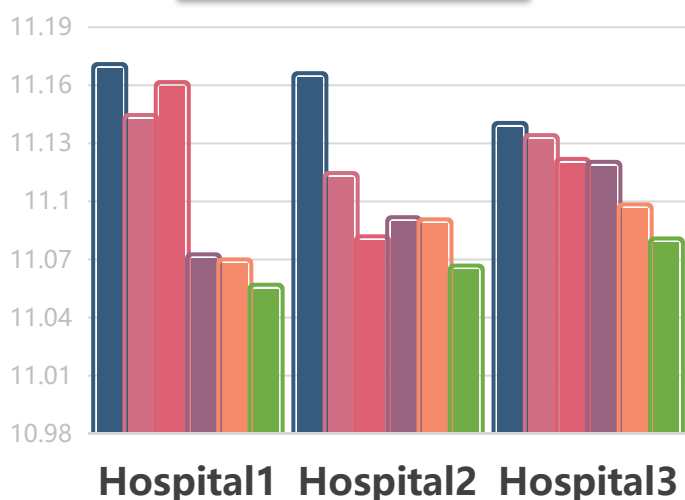

**ASD RH AVERAGE**

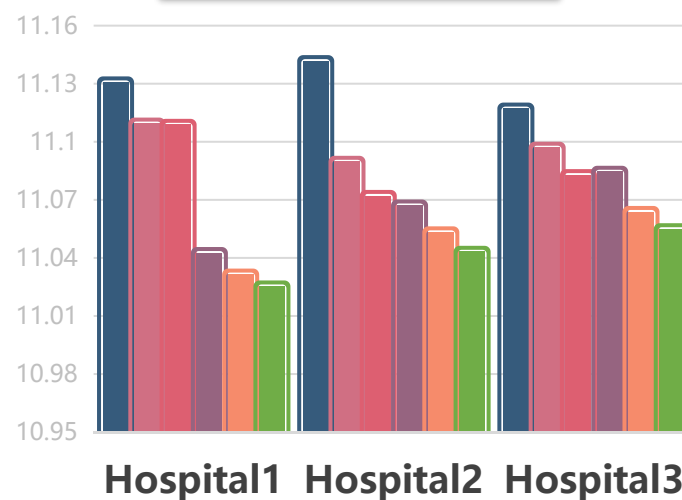

■ DGN 
 ■ RandDGN (Ours) 
 ■ MetaDGN (Ours) 
 ■ FedDGN 
 ■ RandFed (Ours) 
 ■ MetaFed (Ours)

**NC RH FOLD 1**

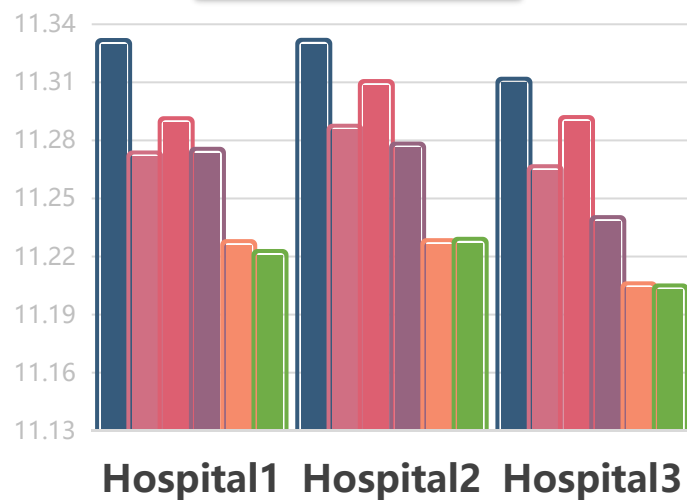

**NC RH FOLD 2**

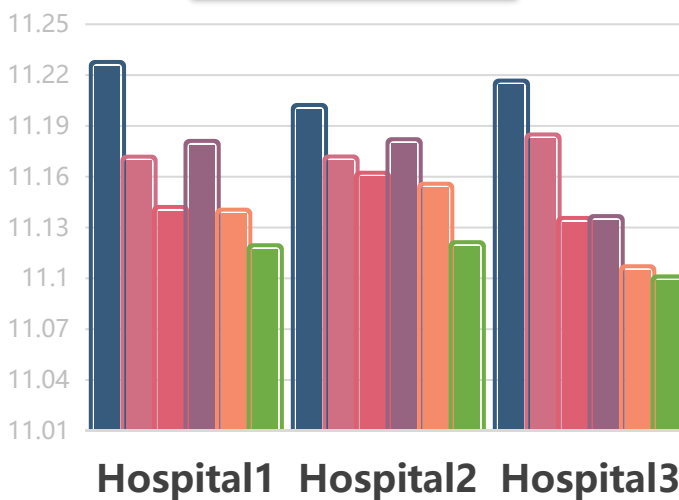

**NC RH FOLD 3**

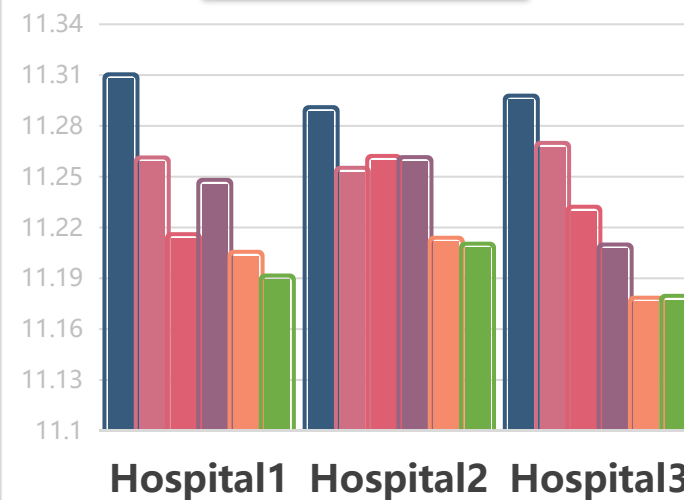

**NC RH FOLD 4**

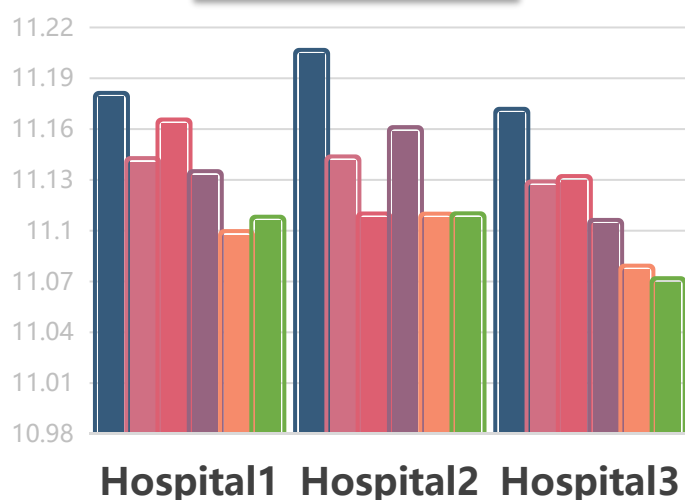

**NC RH AVERAGE**

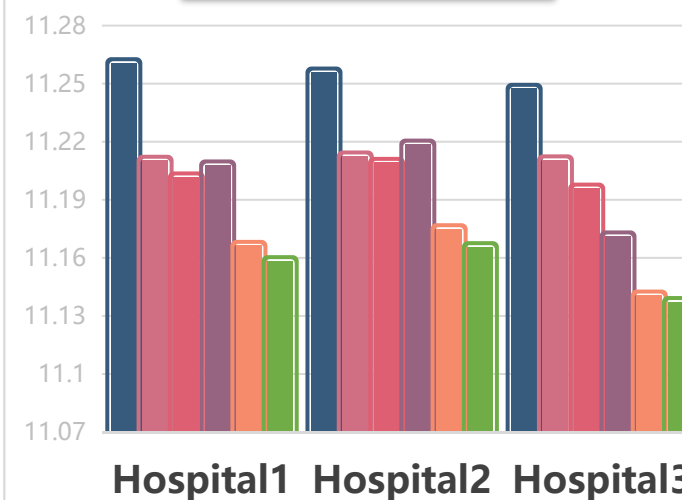

11.28

11.25

11.22

11.19

11.16

11.13

11.1

11.07

- DGN
- RandDGN(Ours)
- MetaDGN(Ours)
- FedDGN
- RandFed(Ours)
- MetaFed(Ours)

Hospital1

Hospital2

Hospital3

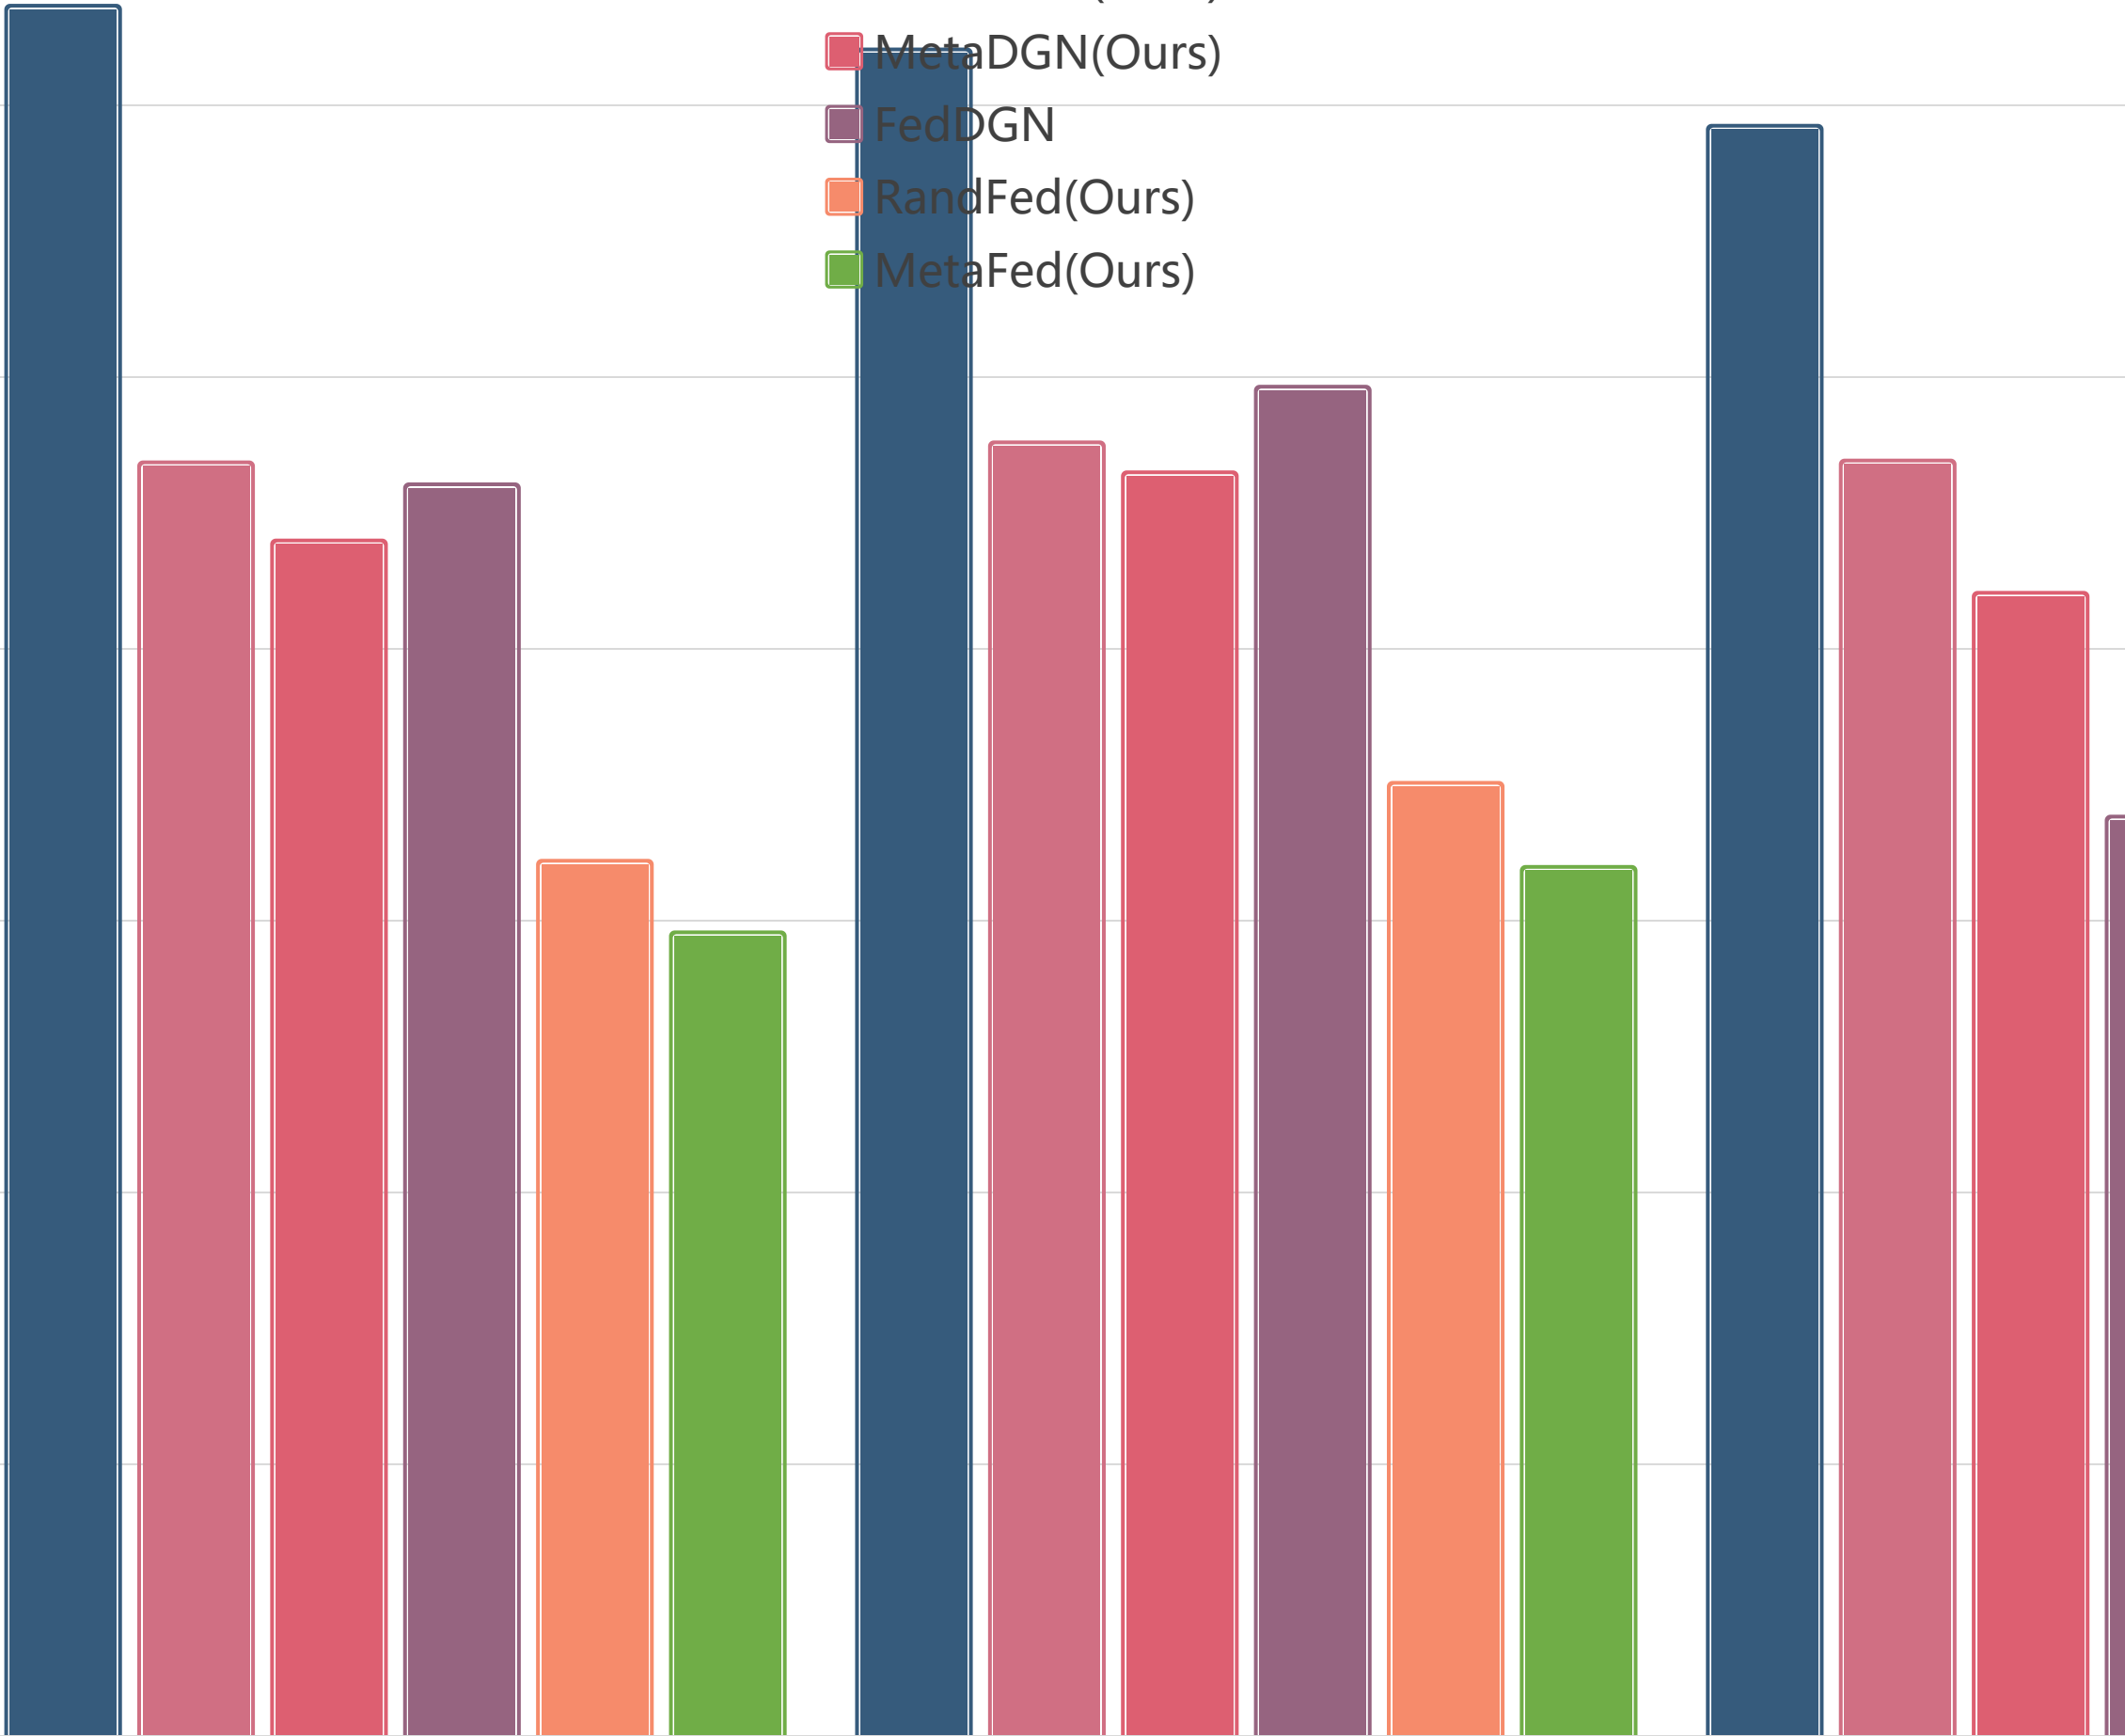

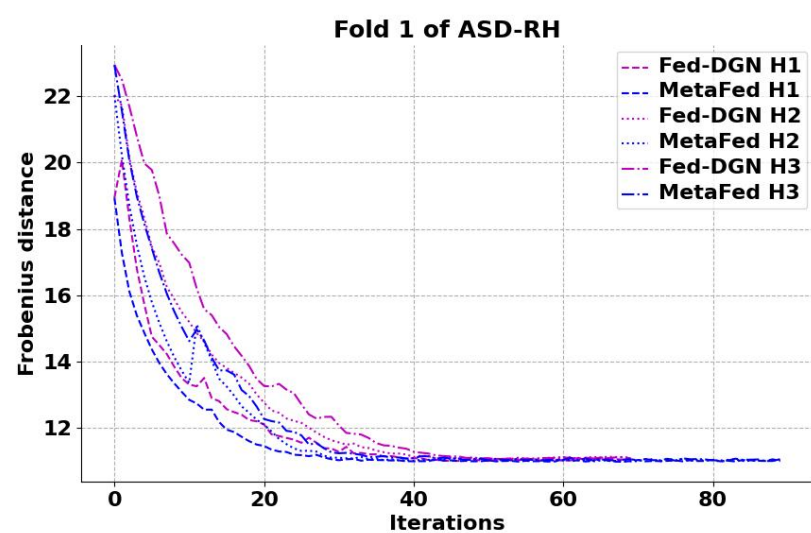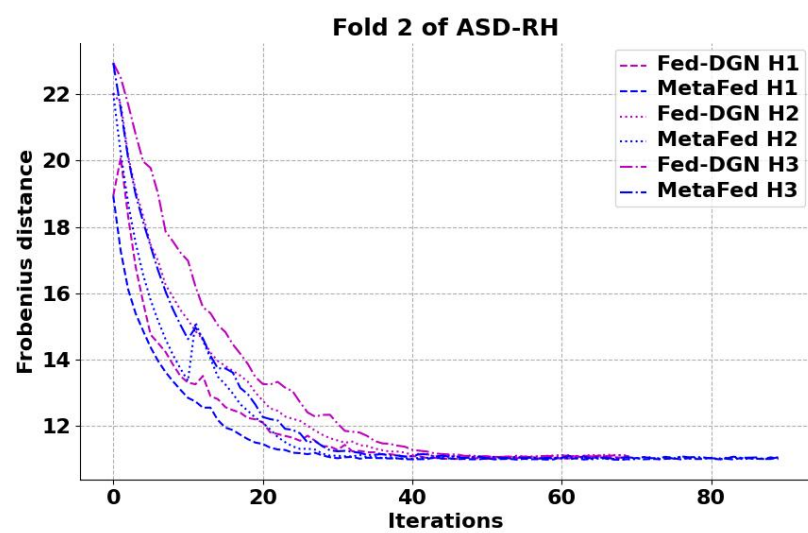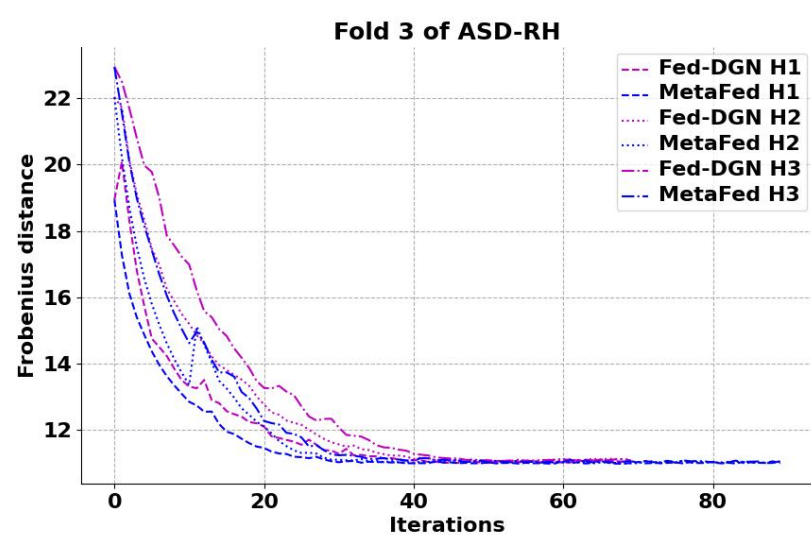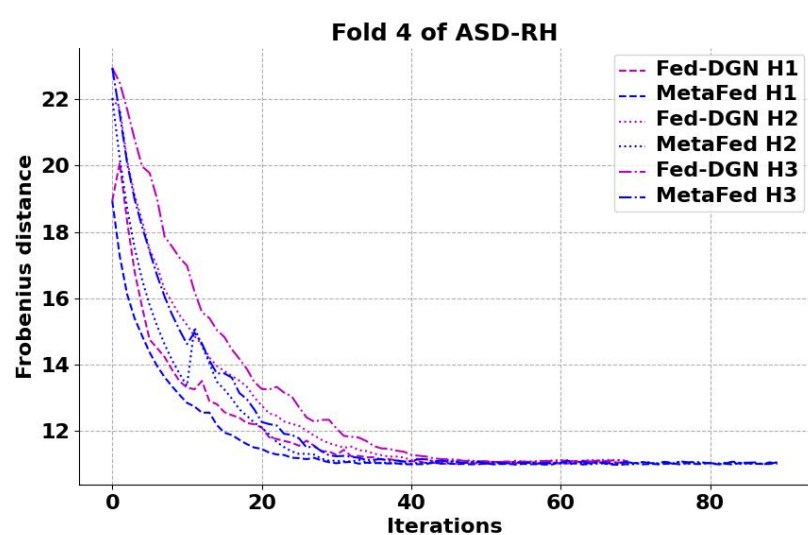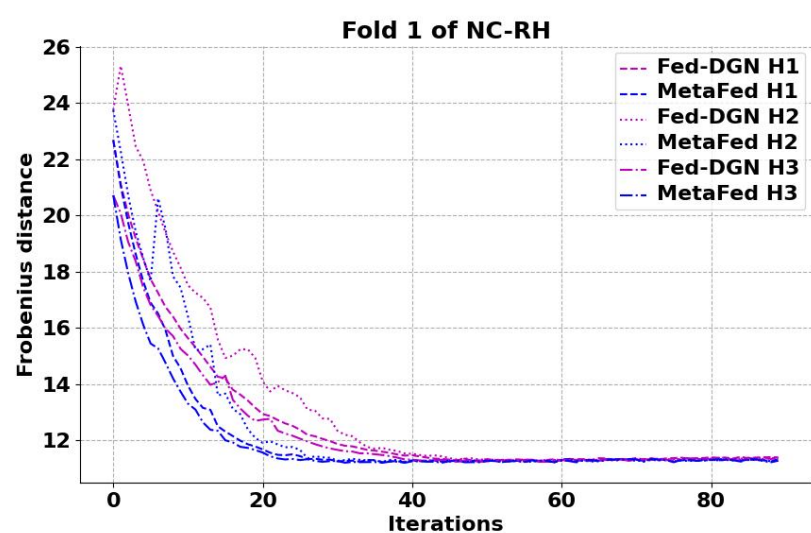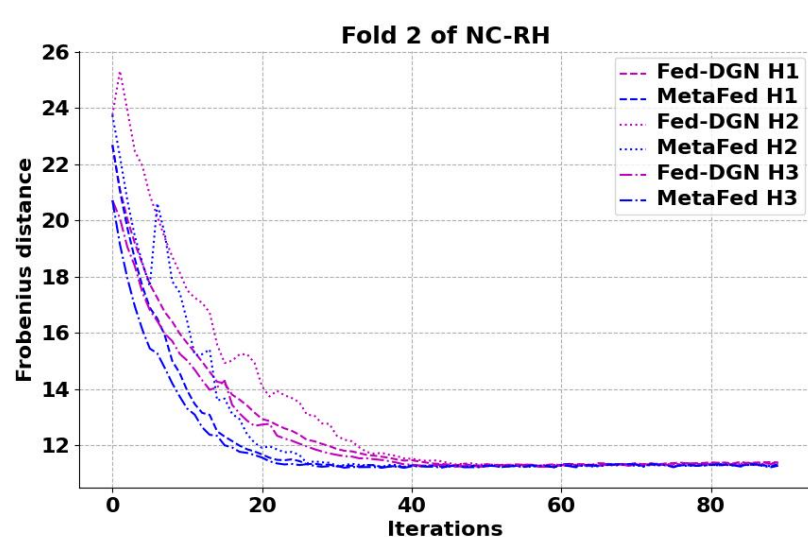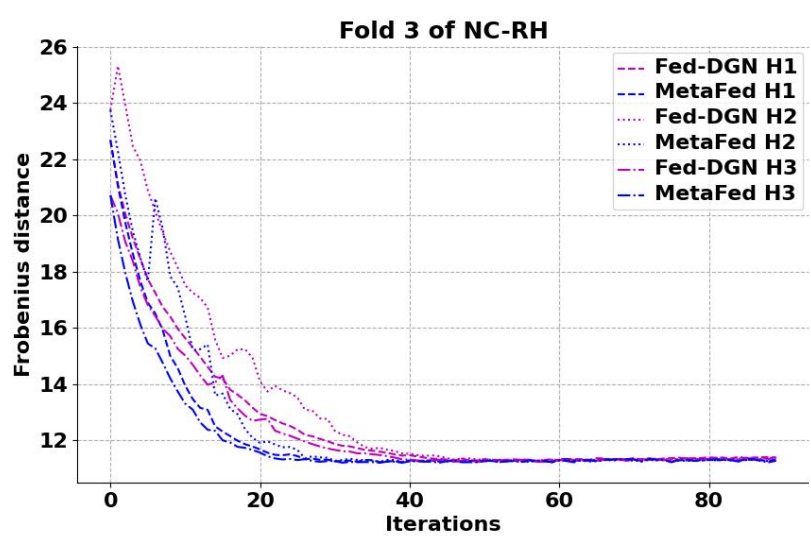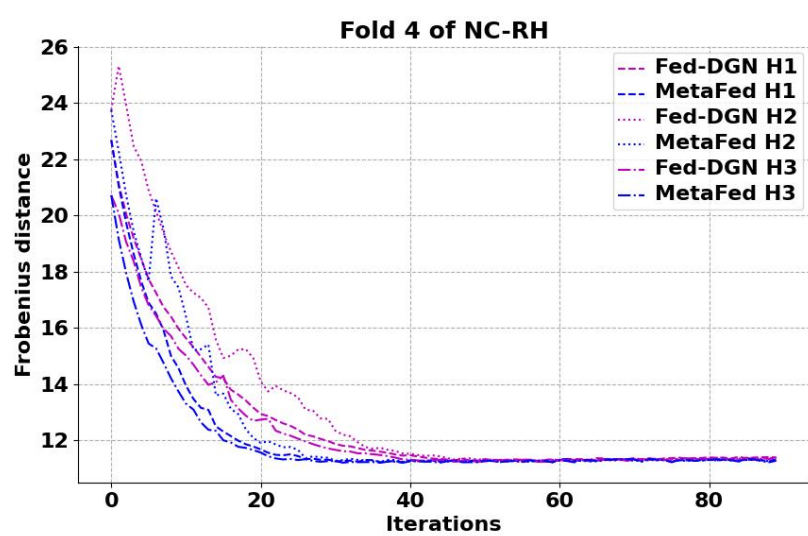

Supplement: Supplementary file 3 [file Supp-Results.pdf]
